# Supplementary material for: VELVET: a noVel Ensemble Learning approach to automatically locate VulnErable sTatements
Source: arXiv:2112.10893 source file (2022-01-13)
Supplement: Supplementary file 1 [file appendix.tex]

\section*{Appendix}

\begin{figure}
    \centering
    \includegraphics[width=\linewidth]{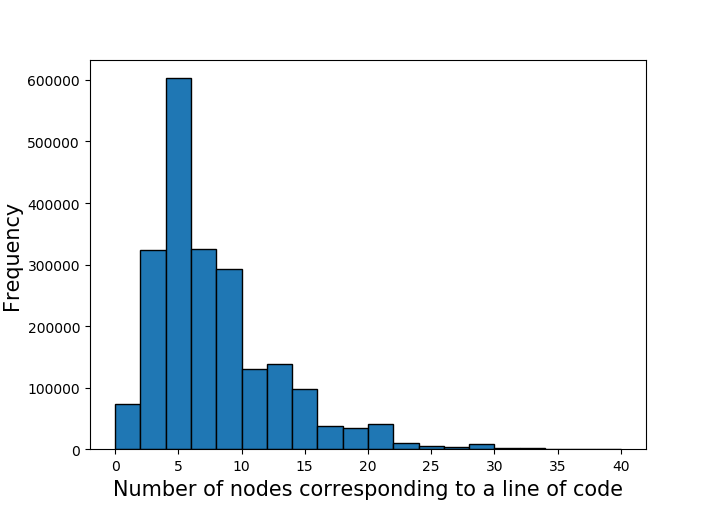}
    \caption{Mean: 7.48, median: 6.0}
    \label{fig:my_label}
\end{figure}
